# Supplementary material for: A Reduction from Multi-Parameter to Single-Parameter Bayesian Contract Design
Source: arXiv:2404.03476 source file (2024-08-22)
Supplement: Supplementary file 1 [file m_appendix.tex]

\newpage
\thispagestyle{empty}

\section*{All are only for reference and will not be included.}

\section*{Proof of $n$ approximation}

Suppose there are $c_1<c_2<\dots <c_T$ types, $T<n$, and $x_{OPT}(c_i) = \arg\max_{k\in[n]}  \{R_k -\gamma_k \bar{\varphi}(c_i)\}$. Suppose $x_{OPT}(c_i)$ are different for $c_i$. $n$ is the number of action.

\begin{align*}
    OPT &= \sum_{i \in [T]}G(c_i)[R_{x_{OPT}(c_i)} - R_{x_{OPT}(c_{i+1})} - c_i(\gamma_{x_{OPT}(c_{i})} - \gamma_{x_{OPT}(c_{i+1})})]
\end{align*}

Let assume $x_{OPT}(c_i) = k+1$ and $x_{OPT}(c_{i+1}) = k-d$ where $d \ge 0$. Then we have
\begin{align*}
& G(c_i)[R_{x_{OPT}(c_i)} - R_{x_{OPT}(c_{i+1})} - c_i(\gamma_{x_{OPT}(c_{i})} - \gamma_{x_{OPT}(c_{i+1})})] \\
& = G(c_i)\Big\{ [R_{k+1} - R_{k} - c_i(\gamma_{k+1} - \gamma_{k})]  + [R_{k} - R_{k-1} - c_i(\gamma_{k} - \gamma_{k-1})] \\
& \quad + \dots + [R_{k-d+1} - R_{k-d} - c_i(\gamma_{k+1-d} - \gamma_{k-d})]\Big\}
\end{align*}
By definition of breakpoints, we know that $c_i \le z_{Wel, k+1}< z_{Wel, k} <\dots <z_{Wel, k-d+1}$, where $z_{Wel}$ defines the breakpoints as the paper.  

Then, there must exist one type $c_i$ and $k$ with $x_{OPT}(c_i) \ge k >x_{OPT}(c_{i+1})$ such that 

\[
G(c_i)[R_{k} - R_{k-1} - c_i(\gamma_{k} - \gamma_{k-1})] \ge \frac{1}{n}OPT
\]

Let $\alpha = \frac{c_i}{z_{Wel, k}}$ be the linear contract. The above becomes
\begin{align*}
& G(\alpha z_{Wel, k})[R_{k} - R_{k-1} - \alpha z_{Wel, k}(\gamma_{k} - \gamma_{k-1})]\\
& = G(\alpha z_{Wel, k})(1-\alpha) (R_k -R_{k-1}) \\
& = G(z_{APX, k}) (1-\alpha) (R_k -R_{k-1})
\end{align*}

\section*{Ironing}
We use the ironing procedure the same as [Elkind2007designing] paper. We only need to compare term $E_{\theta}[c_{\pi(\theta)} \phi(\theta)]$ (note that $c_{\pi(\theta)}$ is decreasing as $\theta$ increases), and get that ironed virtual cost is smaller thus welfare is larger.

\section*{Note for tie-breaking in section 5 main theorem with case analysis}

We can see that by construction 
\[
\theta_{k+1}\cdot (c_{\pi(\theta_k)} - c_{\pi(\theta_{k+1})} )\ge z^{\theta_k} - z^{\theta_{k+1}} = \theta_k\cdot (c_{\pi(\theta_k)}  - c_{\pi(\theta_{k+1})}).
\]
where the right-hand side is binding in the optimal solution. and $z^{\theta_K} = \theta_K c_{a(\theta_K)}$. 

If $\theta_k =0$, optimal action $a$ will be the one with largest $R_a$. Hence, no tie-breaking problem.

For $\theta_k >0$. First, no agent of $\theta_k$ will choose not induced action $\hat{a}$ for tie breaking.
That is $z^{\theta_k} - \theta_{k} c_{a(\theta_k)} = 0 - \theta_k c_{\hat{a}}$. The only possibility is $c_{\hat{a}} = 0$. If $R_{\hat{a}} - 0> R_{a(\theta_k)} -z^{\theta_k}$, then by the maximum virtual welfare action choosing rule, $R_{a(\theta_k)} -z^{\theta_k}  = R_{a(\theta_k)} -z^{\theta_k} +  z^{\theta_k} - \theta_{k} c_{a(\theta_k)} > R_{a(\theta_k)} -z^{\theta_k} +  z^{\theta_k} - \phi(\theta_{k}) c_{a(\theta_k)} = R_{a(\theta_k)}  - \phi(\theta_{k}) c_{a(\theta_k)} \ge R_{\hat{a}} - \phi(\theta_k) c_{\hat{a}} = R_{\hat{a}}$, contradiction.

$\theta_k$ will not choose any action $a(\theta_{k+j})$ for $j>1$. For example, let $j=2$. If $z^{\theta_k} - \theta_k c_{a(\theta_k)} = z^{\theta_{k+2}} - \theta_k c_{a(\theta_{k+2})}$. We know by construction $z^{\theta_k} - \theta_k c_{a(\theta_k)} = z^{\theta_{k+1}} - \theta_k c_{a(\theta_{k+1})}$, and $z^{\theta_{k+1}} - z^{\theta_{k+2}} = \theta_{k+1} (c_{a(\theta_{k+1})}  -  c_{a(\theta_{k+2})})$. Actually, $z^{\theta_{k+1}} - \theta_k c_{a(\theta_{k+1})} > z^{\theta_{k+2}} - \theta_k c_{a(\theta_{k+2})}$, that is $z^{\theta_{k+1}} - z^{\theta_{k+2}} = \theta_{k+1} (c_{a(\theta_{k+1})}  -  c_{a(\theta_{k+2})})  > \theta_k c_{a(\theta_{k+1})}  - \theta_k c_{a(\theta_{k+2})}$, which must hold unless $c_{a(\theta_{k+1})}  =  c_{a(\theta_{k+2})}$. Hence, we only need to consider $\theta_{k+1}$. By binding constraint, we only need to show $R_{a(\theta_k)} - z_{\theta_k} \ge R_{a(\theta_{k+1})} - z_{\theta_{k+1}}$. Actually, $R_{a(\theta_k)} - \phi(\theta_{k})c_{a(\theta_k)} \ge R_{a(\theta_{k+1})} - \phi(\theta_k) c_{a(\theta_{k+1})}$, then $R_{a(\theta_k)} - (\theta_{k})c_{a(\theta_k)} \ge R_{a(\theta_{k+1})} - (\theta_k) c_{a(\theta_{k+1})}$ since $c_{a(\theta_k)} \ge c_{a(\theta_{k+1})}$. Then $R_{a(\theta_k)} - z_{\theta_k} + z_{\theta_k} - (\theta_{k})c_{a(\theta_k)} \ge R_{a(\theta_{k+1})}- z_{\theta_{k+1}} + z_{\theta_{k+1}} - (\theta_k) c_{a(\theta_{k+1})}$.

If $\theta_k$ chooses $a(\theta_{k-1})$ for tie breaking, by  $z^{\theta_k} - \theta_k c_{a(\theta_k)} = z^{\theta_{k-1}} - \theta_k c_{a(\theta_{k-1})}$ and the binding IC $z^{\theta_{k-1}} - \theta_{k-1} c_{a(\theta_{k-1})} = z^{\theta_k}-\theta_{k-1} c_{a(\theta_{k})} $, then $c_{a(\theta_k)} = c_{a(\theta_{k-1})}$. No tie-breaking problem. For $j>2$. If $z^{\theta_k} - \theta_k c_{a(\theta_k)} = z^{\theta_{k-j}} - \theta_k c_{a(\theta_{k-j})}$. Because $z^{\theta_k} - \theta_k c_{a(\theta_k)} \ge z^{\theta_{k-g}} - \theta_k c_{a(\theta_{k-g})}$ for $g < j$. We know $z^{\theta_{k-j}} - \theta_k c_{a(\theta_{k-j})} \le z^{\theta_{k-g}} - \theta_k c_{a(\theta_{k-g})}$, that is $z^{\theta_{k-j}}- z^{\theta_{k-g}} \le  \theta_k c_{a(\theta_{k-j})}   - \theta_k c_{a(\theta_{k-g})}$ which must satisfy since $z^{\theta_{k-j}}- z^{\theta_{k-g}} \le \theta_{k-g} (c_{a(\theta_{k-j})}   -  c_{a(\theta_{k-g})}) \le \theta_k c_{a(\theta_{k-j})}   - \theta_k c_{a(\theta_{k-g})}$, where the first inequality is by IC and the second is by $\theta_{k-g} < \theta_k$. Then, $z^{\theta_k} - \theta_k c_{a(\theta_k)} \ge z^{\theta_{k-g}} - \theta_k c_{a(\theta_{k-g})} \ge z^{\theta_{k-j}} - \theta_k c_{a(\theta_{k-j})}$. Then, all hold equality. That is $c_{a(\theta_k)} = c_{a(\theta_{k-j})}$. No tie-breaking problem.
